# Supplementary material for: A Unified Statistical Framework for Single Cell and Bulk RNA Sequencing Data
Source: arXiv:1609.08028 source file (2017-10-19)
Supplement: Supplementary file 1 [file SC-supplement.tex]

\documentclass[aoas, preprint]{imsart}
\arxiv{arxiv:1606.00252}
\includeonly{supplement}

% packages
\RequirePackage[OT1]{fontenc}
\usepackage{subcaption, adjustbox} 
\usepackage{amsthm, amsmath, amsfonts, enumerate, mathtools, natbib}
\RequirePackage[colorlinks, citecolor=blue, urlcolor=blue]{hyperref}
\usepackage{verbatim} % for comment block
\usepackage{imsart}
\usepackage[dvipsnames]{xcolor}

% Ref style
\usepackage{cleveref}
\crefformat{equation}{(#2#1#3)} % \cref{eq1} 
\crefrangeformat{equation}{(#3#1#4) to~(#5#2#6)} % \crefrange{eq1}{eq5}
\crefformat{enumi}{step~#2#1#3} % \cref{step1} 
\crefrangeformat{enumi}{steps~#3#1#4~--~#5#2#6}
\crefformat{figure}{Figure~#2#1#3}

% command definitions
\startlocaldefs
\numberwithin{equation}{section}
\theoremstyle{plain}

\captionsetup[subfigure]{labelfont=footnotesize}

\long\def\@makecaption#1#2{%
  \vskip\abovecaptionskip
  \footnotesize
  \sbox\@tempboxa{\itshape\textsc{#1}. #2}%
  \ifdim \wd\@tempboxa >\hsize
    \itshape\textsc{#1}. #2\par
  \else
    \global \@minipagefalse
    \hb@xt@\hsize{\hfil\box\@tempboxa\hfil}%
  \fi
  \vskip\belowcaptionskip}

\long\def\@makecaption#1#2{%
  \vskip\abovecaptionskip
  \figurecaption@size
  \sbox\@tempboxa{{\figurename@size #1}\figurename@skip #2}%
  \ifdim \wd\@tempboxa >\hsize
    {\figurename@size #1}\figurename@skip #2\par
  \else
    \global \@minipagefalse
    \hb@xt@\hsize{\hfil\box\@tempboxa\hfil}%
  \fi
  \vskip\belowcaptionskip}

\setattribute{figurecaption}{size}{\footnotesize\itshape}
\setattribute{figurename}   {size}{\scshape}
\setattribute{figurename}   {skip}{.~~}

\def\@floatboxreset{%
        \reset@font
        \@setminipage
        \singlespacing
        \footnotesize
        \centering
}

\endlocaldefs

%% supplement labels
\newcommand{\beginsupplement}{%
        \setcounter{table}{0}
        \renewcommand{\thetable}{S\arabic{table}}%
        \setcounter{figure}{0}
        \renewcommand{\thefigure}{S\arabic{figure}}%
         \setcounter{section}{0}
        \renewcommand{\thesection}{S\arabic{section}}%
}

% table spacing
\bgroup
 % table vertical spacing; 1 is the default
 % bf without changing the table width

% begin document
\begin{document}

%% comment out main if don't want the full reference list
\include{main}

\begin{frontmatter}

\title{Supplemental Document for ``A Unified Statistical Framework for Single Cell and Bulk RNA Sequencing Data"}
\runtitle{}

%% authors
\begin{aug}
\author{\fnms{Lingxue} \snm{Zhu}\thanksref{t1}\ead[label=e1]{lzhu@cmu.edu}},
\author{\fnms{Jing} \snm{Lei}\thanksref{t1}\ead[label=e2]{jinglei@andrew.cmu.edu}},
\author{\fnms{Bernie} \snm{Devlin}\thanksref{t2}\ead[label=e3]{devlinbj@upmc.edu}}
\and
\author{\fnms{Kathryn} \snm{Roeder}\corref{}\thanksref{t1}\ead[label=e4]{roeder@andrew.cmu.edu}}

\affiliation{Carnegie Mellon University\thanksmark{t1}
and
University of Pittsburgh\thanksmark{t2}}

\address{Department of Statistics\\
Carnegie Mellon University\\
5000 Forbes Avenue\\
Pittsburgh, Pennsylvania 15213\\
USA\\
\printead{e1}\\
\phantom{E-mail:\ }\printead*{e2}\\
\phantom{E-mail:\ }\printead*{e4}}

\address{Department of Psychiatry and Human Genetics\\
University of Pittsburgh School of Medicine\\
3811 O'Hara Street\\
Pittsburgh, Pennsylvania 15213\\
USA\\
\printead{e3}}

\runauthor{L. Zhu, J. Lei, B. Devlin and K. Roeder}
\end{aug}

\begin{abstract}
This document provides supplementary material to the article ``A Unified Statistical Framework for Single Cell and Bulk RNA Sequencing Data"
written by the same authors.
\end{abstract}

\end{frontmatter}

\beginsupplement
\input{Appendix}

\bibliography{singlecell}
\bibliographystyle{imsart-nameyear}

\end{document}
